# Supplementary material for: Computational homogenization of phase-field fracture
Source: arXiv:2312.12776 source file (2023-12-20)
Supplement: Supplementary file 1 [file sec_appendix.tex]

Hallo Welt.
